# Supplementary material for: Relation between interface symmetry and propagation robustness along domain walls based on valley topological photonic crystals
Source: arXiv:2408.10294 source file (2024-08-19)
Supplement: Supplementary file 1 [file suppmat_sub.pdf]

# Supplemental Materials for Relation between interface symmetry and propagation robustness along domain walls based on valley topological photonic crystals

Gaëtan Lévêque and Yan Pennec

*Univ. Lille, Institut d'Electronique,  
de Micro-électronique et de Nanotechnologie  
(IEMN, CNRS-8520), Cité Scientifique,  
Avenue Poincaré, 59652 Villeneuve d'Ascq, France\**

Pascal Szriftgiser and Alberto Amo

*Univ. Lille, CNRS, UMR 8523-PhLAM-Physique des  
Lasers Atomes et Molécules, F-59000 Lille, France*

(Dated: August 18, 2024)

---

\* [gaetan.leveque@univ-lille.fr](mailto:gaetan.leveque@univ-lille.fr)

## I. EFFECT OF THE PERMUTATIONS ON THE LATTICE

The permutation  $(\beta, \gamma, \alpha)$  changes  $\alpha$  into  $\beta$ ,  $\beta$  into  $\gamma$  and  $\gamma$  into  $\alpha$ .

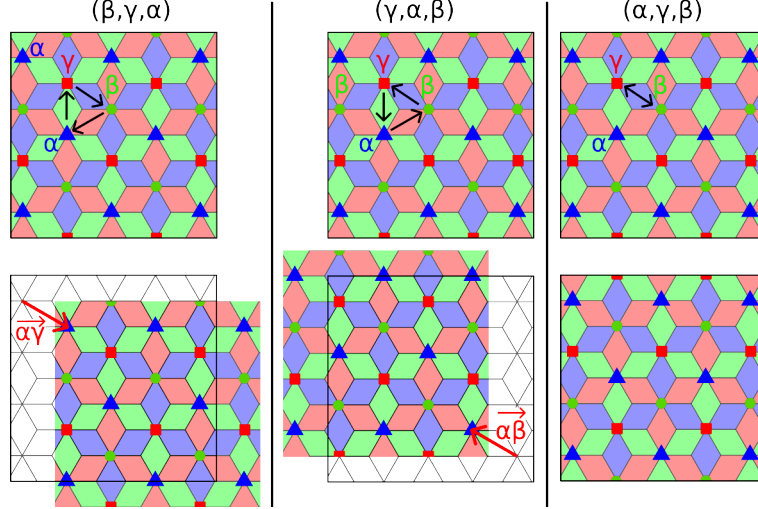

The cyclic permutation  $(\beta, \gamma, \alpha)$  (left panel) translates the lattice by either  $\vec{\alpha\gamma}$ ,  $\vec{\beta\alpha}$  or  $\vec{\gamma\beta}$ , the permutation  $(\gamma, \alpha, \beta)$  (middle panel) by either  $\vec{\alpha\beta}$ ,  $\vec{\beta\gamma}$  or  $\vec{\gamma\alpha}$ , while the transposition  $(\alpha, \gamma, \beta)$  (right panel) exchanges the  $\beta$  and  $\gamma$  axes (green and red diamonds) while keeping the  $\alpha$  axes unchanged (blue diamonds).

## II. CONSTRUCTIONS OF BEARDED INTERFACES

Panels (a) and (b) of Fig. S1 correspond to cases where the original (top) and image (bottom) lattices differ by a transposition: they are mirror-symmetric (up to a sub-lattice translation) and one of the three sub-lattices of rotation axes is left unchanged. We consider first the super-cell pictured on the top-left part of panel (a). The interface (black thick line) connects  $\alpha$  and  $\beta$  sites of the original lattice, and  $\beta$  and  $\alpha$  sites of the image lattice. The original lattice is then transformed into the image lattice by exchanging  $\alpha$  and  $\beta$  sub-lattices, while keeping  $\gamma$  sites in place, or applying the transposition  $(\beta, \alpha, \gamma)$ . The resulting interface, which presents a glide-mirror symmetry materialized by the dashed line, is the analog of the bearded interface between two symmetric honeycomb lattices. For each of the three couples of sites connected by the solid line, there are two possible configurations of sub-lattices, leading to six distinct interfaces pictured in the six illustrations. Associated dispersion diagrams show that only four interfaces ( $i$ ,  $ii$ ,  $iv$ ,  $v$ ) out of six sustain edge modes. As

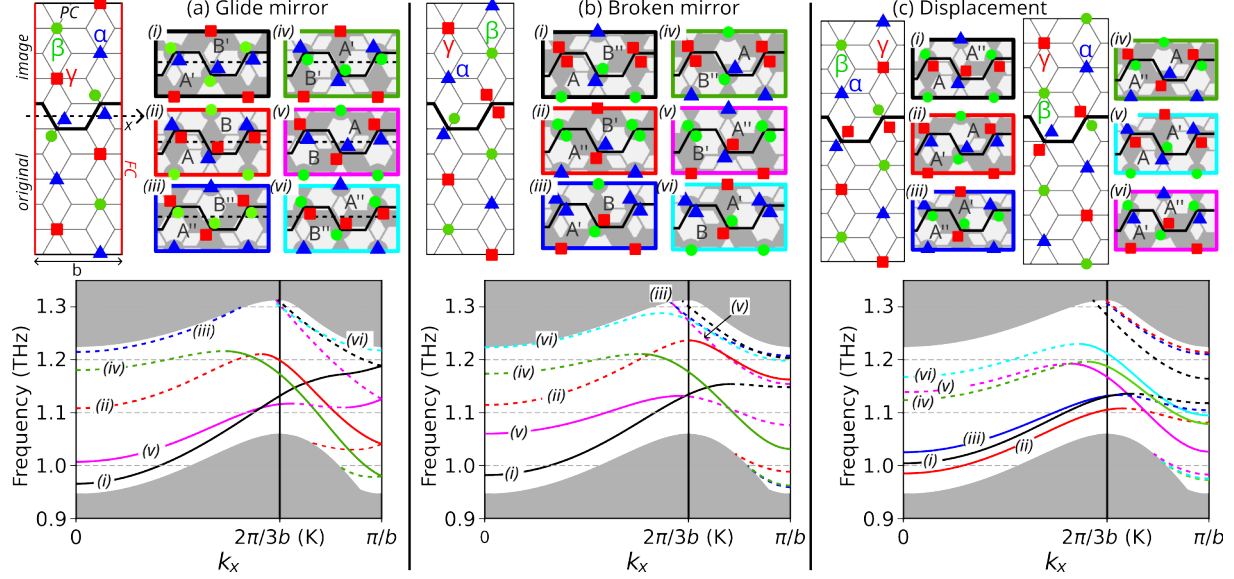

FIG. S1. (a) Top: super-cell of a typical interface obtained by a transposition with glide-mirror symmetry between original and image lattices, and corresponding six possible interfaces ; bottom: dispersion diagrams of the six interfaces. A solid line indicates robust protection against back-reflection at sharp bends, a dashed line corresponding to strong reflection. (b) Same as (a) but for a transpositions breaking the glide-mirror symmetry. (c): Same as (a) but for cyclic permutations. (d) Amplitude profiles of the edge-modes propagating along a Z-interface, for selected frequencies and interfaces.

expected due to the glide-mirror symmetry, the dispersion curves are all folded at the edges of the first Brillouin zone of the interface,  $k_x = \pm\pi/b$ , leading to a degeneracy point. In the second class of edges, corresponding to panel (b), the original and image lattices are related by a transposition which leaves unchanged one of the two sub-lattices having rotation axes along the interface. On the super-cell plotted in the top left part, the  $\alpha$  sub-lattice is unchanged, while the  $\beta$  and  $\gamma$  axes are exchanged. As for the previous case, there are six possible edges with similar transformation. However, those so-called "broken-mirror" interfaces does not have a glide-mirror symmetry, and the four obtained edge-modes ( $i$ ,  $iii$ ,  $v$ ,  $vi$ ) are all gaped at  $k_x = \pm\pi/b$ . In the last case, panel (c), the original and image lattices are related by a cyclic permutation of the three sub-lattices of rotation axes, equivalent to a translation. There are two families of three interfaces depending on whether the cyclic permutation is in one direction or the other. For example, the left and right super-cells on the top part of panel (c) correspond respectively to the  $(\beta, \gamma, \alpha)$  and  $(\gamma, \alpha, \beta)$  permutations.

For each direction, there are three configurations leading again to six distinct interfaces.

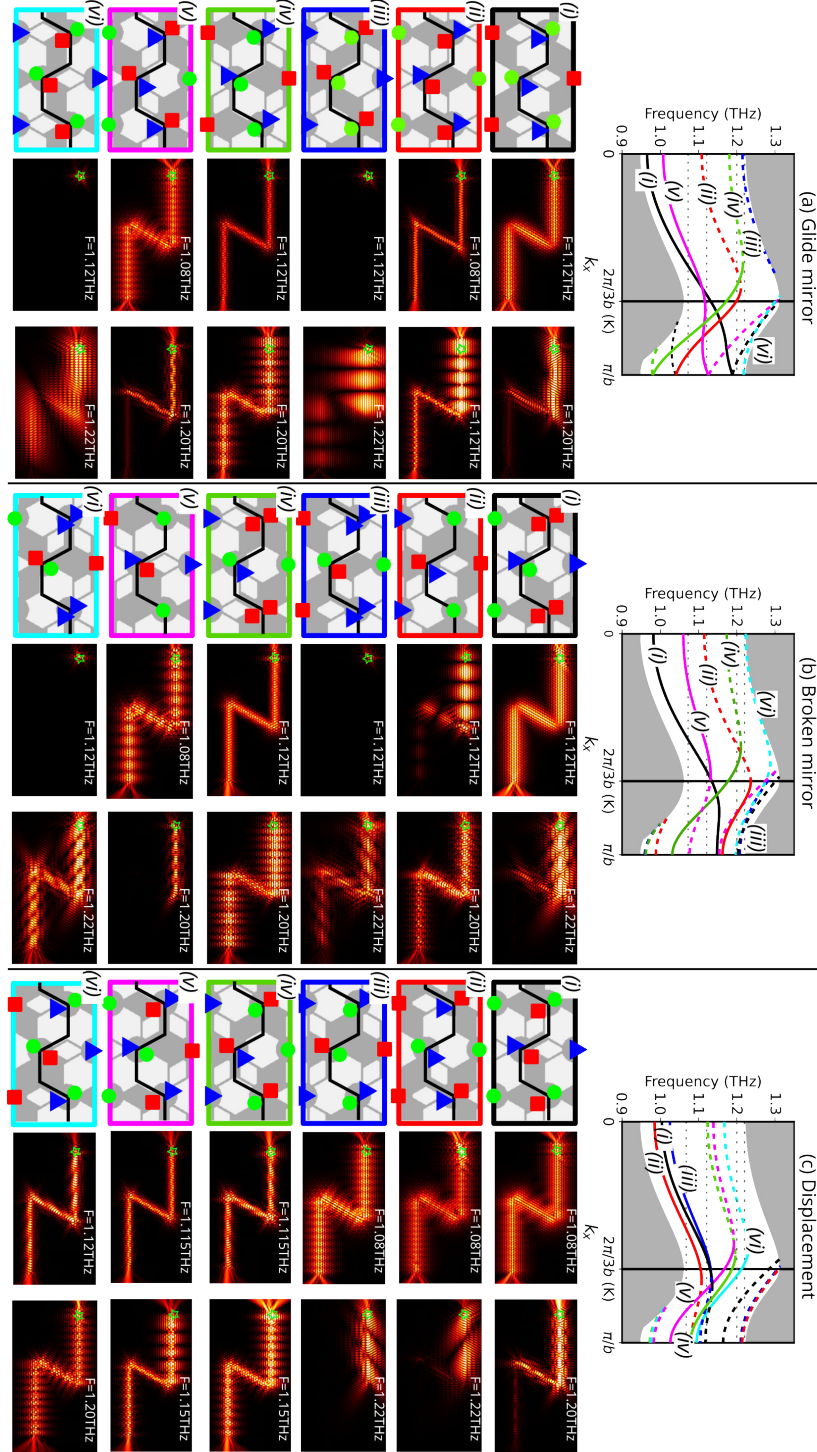

FIG. S2. Dispersion relations and distribution of the magnetic field amplitude for the edge-modes propagating along the 18 identified interfaces, through two  $120^\circ$  bends.

### III. INTERFACES CORRESPONDENCES

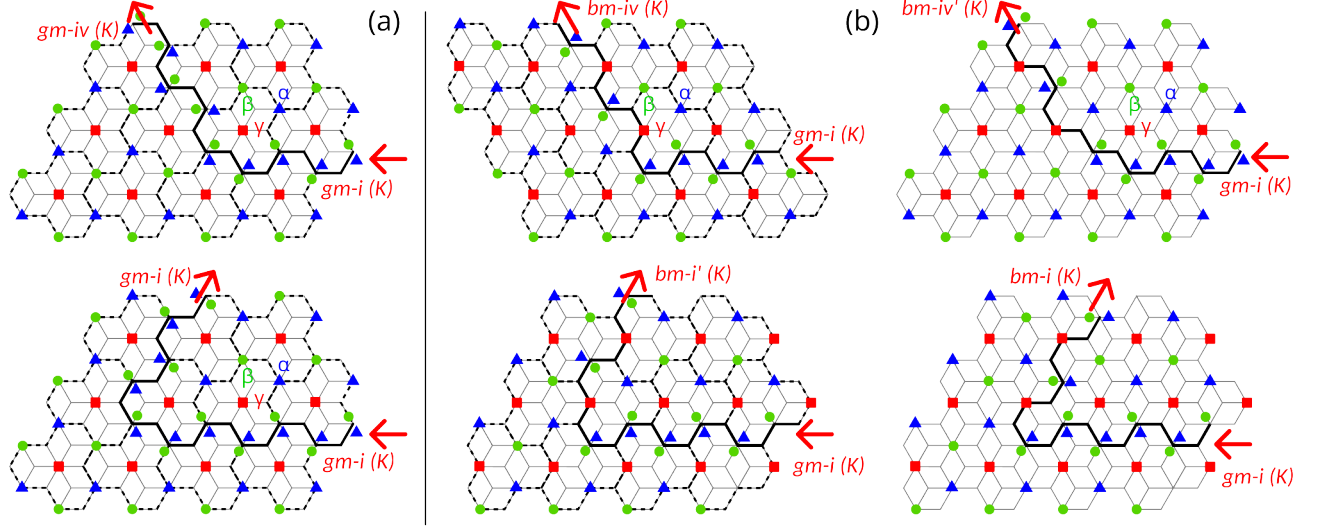

FIG. S3. Relations between interfaces with  $120^\circ$  or  $60^\circ$  depending on the shape of the unit cell (dashed black line). (a) The unit cell conserves the interface symmetry. (b) The unit cell changes the interface symmetry. Primed and un-primed interfaces are traveled in opposite directions.

#### IV. EDGE-MODES SIMULATIONS FOR 60° AND 90° CORNERS

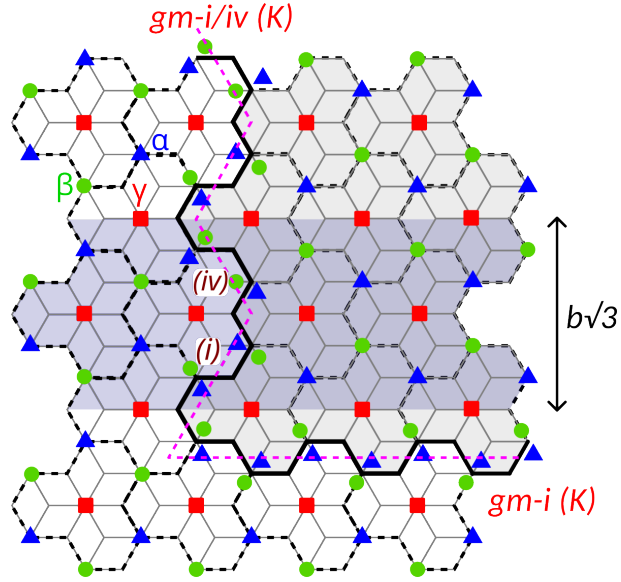

FIG. S4. Shape of a 90° bend connecting, for glide-mirror interfaces, a (i)-type  $\Gamma K$  interface and a (i-iv)-type  $\Gamma M$  interface. In gray is highlighted the supercell used to compute the dispersion curve of a  $\Gamma M$  edge-mode, with period  $b\sqrt{3}$ .

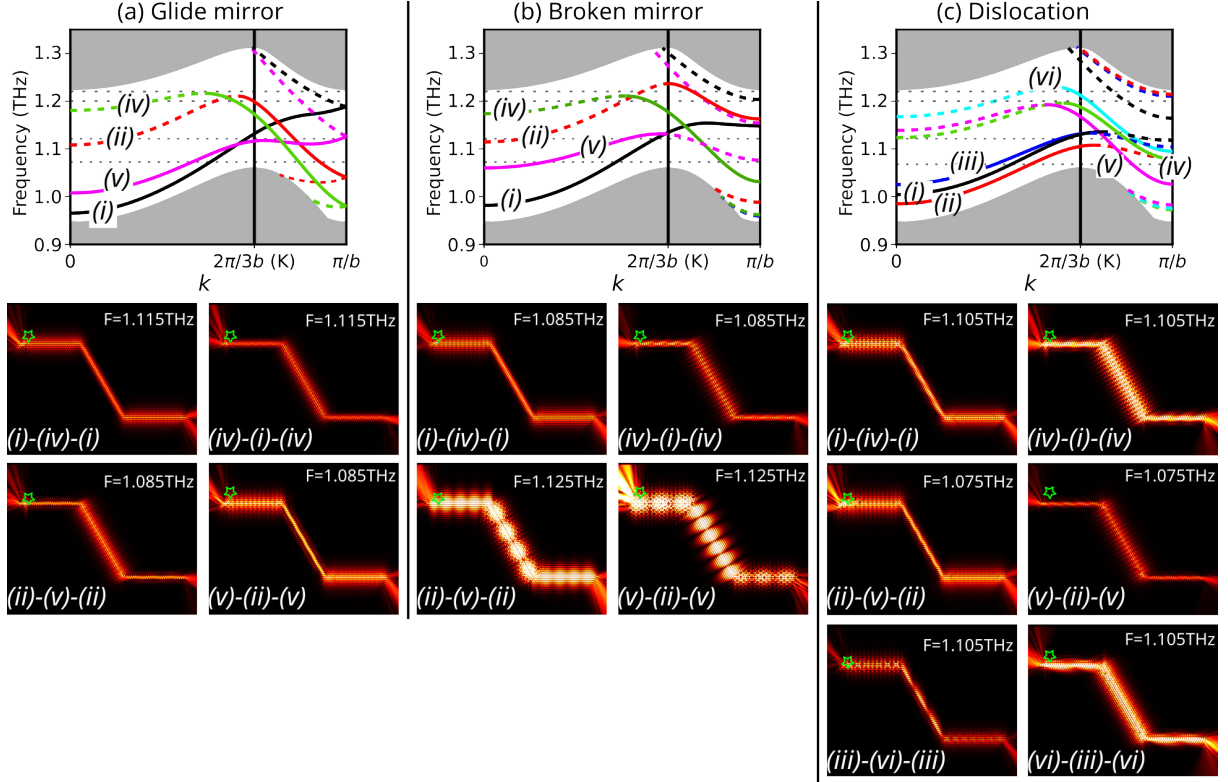

FIG. S5. Dispersion relations and distribution of the magnetic field amplitude for the edge-modes propagating along the 14 identified interfaces sustaining edge modes, through two  $60^\circ$  bends.

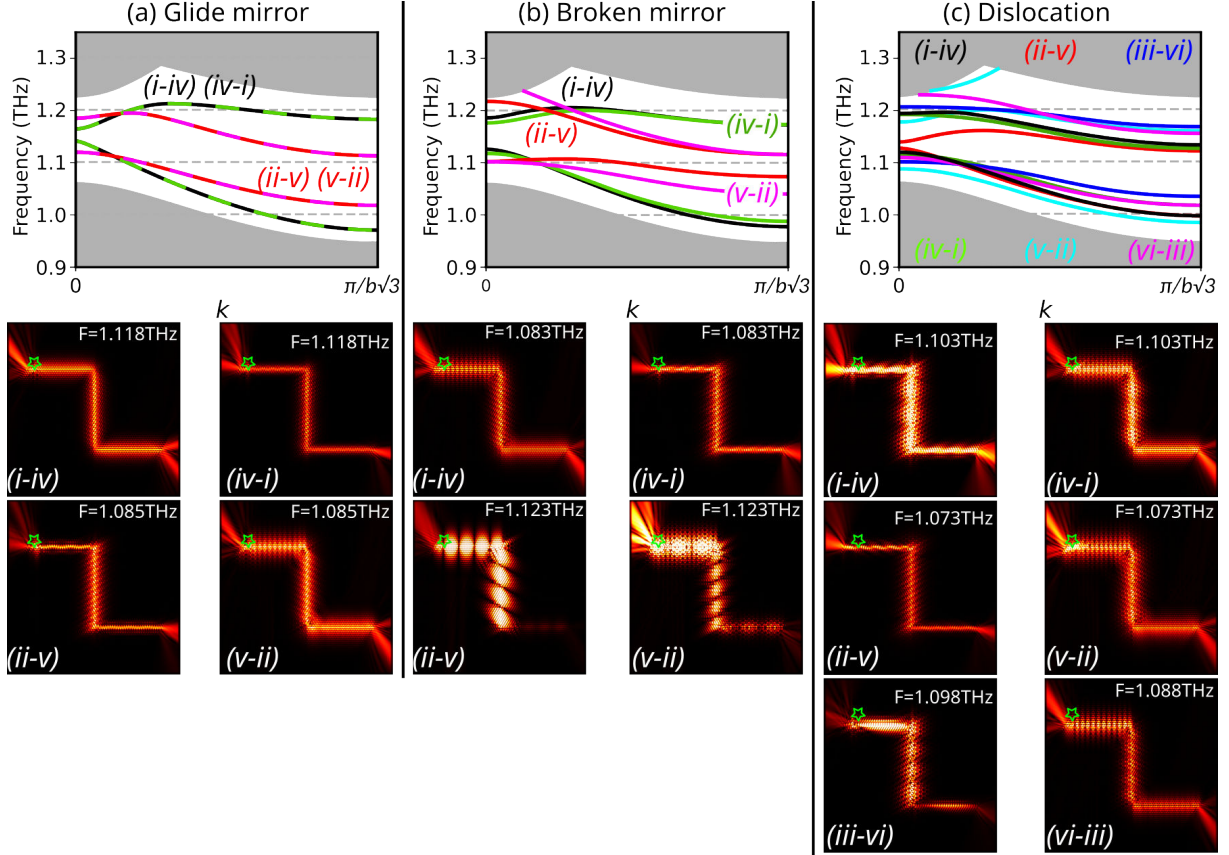

FIG. S6. Dispersion relations of  $\Gamma$ M interfaces, and distribution of the magnetic field amplitude for the edge-modes propagating along the 14 identified interfaces sustaining edge modes, through two  $90^\circ$  bends.

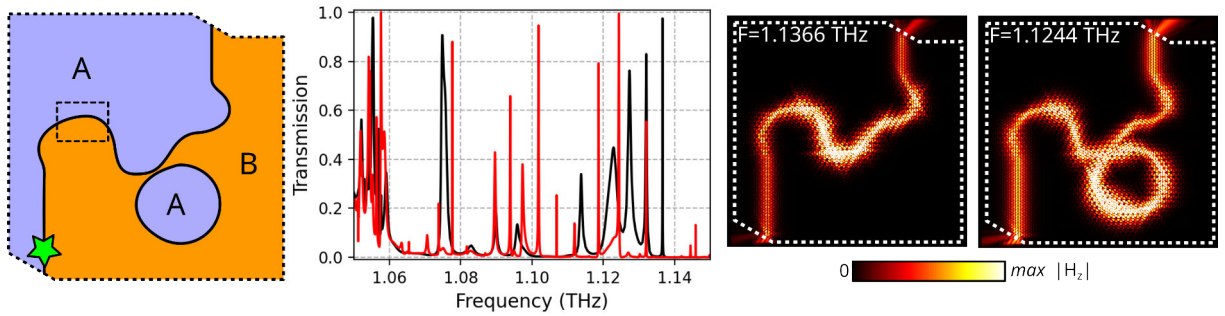

FIG. S7. Transmission of a broken-mirror edge-mode through an edge with arbitrary shape between lattice  $A$  and  $B$ , built on  $bm-i$  and  $bm-iv$  interfaces. The source is located at the position of the green star. Transmission spectra are plotted without (black) and with (red) resonator. Magnetic field amplitude distributions correspond to selected frequencies without and with resonator.
